# Supplementary material for: Federated Learning as a Network Effects Game
Source: arXiv:2302.08533 source file (2023-02-16)
Supplement: Supplementary file 1 [file appendix-linear-regression.tex]

\section{Federated Learning model for linear regression}
\paragraph{Setup}
There is a fixed set of $M$ clients wanting to solve a common learning problem of estimating the global parameter $\theta$ through linear regression. Each client $i$ has a fixed number of samples $n_i$ and a cost $c_i$. First, each client $i$ draws their mean parameter i.i.d from a common prior $\mu_i \sim \calN(\theta, \Sigma_\mu)$ where $\mu_i$ is a $D-$dimensional vector. \dnedit{They also draw their scalar variance parameter $\epsilon^2_j \sim \calN(\mu_\epsilon, \sigma_\epsilon)$.}
We assume that each coordinate $\mu_i^{d}$ is drawn independently of the others. Then, each client draws $n_j$ training samples from their own input distribution $X_i \sim \calX_i$ such that $\E_{x \sim \calX_i}[x^\top x] = \Sigma_i$. The clients observes noisy labels $Y_i \sim \calN(X_i^\top \mu_i, \epsilon^2_i)$. We use $\eta_i$ to denote the noise vector of length $D$ such that $Y_i = X_i^\top \mu_i + \eta_i$. Each client uses ordinary least squares (OLS) to compute the estimates of their parameters. We assume that the matrix $X_i^\top X_i$ is invertible for each client $i$ so they can perform OLS, which means each column of $X_i^\top X_i$ is linearly independent. Furthermore, we assume that the local samples $X_i$ are $0$-mean $D$-dimensional vector. Formally, the local estimate $w_i$ for client $i$ using their own data samples is:
\begin{equation*}
    w_i = (X_i^\top X_i)^{-1} X_i^\top Y_i = (X_i^\top X_i)^{-1} X_i^\top (X_i \theta_i + \eta_i)
\end{equation*}
The expected error for an estimate $w_i$ is determined by the expectation of difference between predicted label and true label for a freshly drawn test point $x$ \citep{modelsharing2020donahue}. Formally, we focus on the following term:
\begin{equation*}
    \E([x^\top w_i - x^\top \theta)^2]
\end{equation*}
where the expectation is taken over four sources of randomness:
\begin{enumerate}
    \item $\E_{(\mu_i, \epsilon_i^2) \sim \calN(\theta, \Sigma_\mu)}$: Drawing the true local mean $\mu_i$ and true local variance $\epsilon_i^2$ from the prior.
    \item $\E_{X_i \sim \calX_i}$: Drawing the training set $X_i$ from the local data distribution $\calX_i$. 
    \item $\E_{Y_i \sim \calN(X_i^\top \mu_i, \epsilon_i^2)}$: Drawing the labels for the training dataset $X_i$.
    \item $\E_{x \sim \calX_i}$: Drawing a new test point $x$ from the data distribution $\calX_i$.
\end{enumerate}
We can calculate the expected error for the local estimator $w_i$ as follows:
\begin{lemma} For linear regression, the expected MSE of local estimation for a player with $n_i$ samples is
\begin{equation*}
    \frac{\mu_\epsilon}{n_i - D - 1} D + \tr[\Sigma_\mu \Sigma_i]
\end{equation*}
\end{lemma}
\begin{proof}
First, we can expand the expected error expression using definition of OLS:
\begin{align*}
    (x^\top \theta - x^\top w_i)^2 &= \left( (x^\top \theta - x^\top \mu_i) + (x^\top \mu_i - x^\top w_i) \right)^2\\
    &= \underbrace{(x^\top \theta - x^\top \mu_i)^2}_{A} + \underbrace{(x^\top \mu_i - x^\top w_i)^2}_{B} + \underbrace{2(x^\top \theta - x^\top \mu_i)(x^\top \mu_i - x^\top w_i)}_{C}
\end{align*}  
We proceed to calculate the expectation of each term separately. For A, we have:
\begin{align*}
    \E[A] &= \E_{\substack{\mu_i \sim \calN(\theta, \Sigma_\mu)\\ x \sim \calX_i}}[(x^\top \theta - x^\top \mu_i)^2]\\
    &= \E_{\substack{\mu_i \sim \calN(\theta, \Sigma_\mu) \\ x \sim \calX_i}}[(\theta - \mu_i)^\top x x^\top(\theta - \mu_i)]\\
    &= \E_{\substack{\mu_i \sim \calN(\theta, \Sigma_\mu) \\ x \sim \calX_i}}[\tr[(\theta - \mu_i)^\top x x^\top (\theta - \mu_i)]\\
    &= \E_{\substack{\mu_i \sim \calN(\theta, \Sigma_\mu) \\ x \sim \calX_i}}[\tr[x^\top (\theta - \mu_i) (\theta - \mu_i)^\top x] \tag{by cyclic trace commute}
\end{align*}
Taking expectation over the drawn local mean $\mu_i$ and using the fact that $\E[\tr[A]] = \tr[\E[A]]$ for any matrix square A, we have:
\begin{align*}
    \E[A] &= \E_{x \sim \calX_i}[\tr[x^\top \Sigma_\mu x]] \\
    &= \E_{x \sim \calX_i}[\tr[\Sigma_\mu x x^\top]]\\
    &= \tr[\Sigma_\mu \Sigma_i]]
\end{align*}
Since $x$ is a $0$-mean $D$-dimensional vector drawn from a multivariate normal distribution, the trace of $x x^\top$ is a sum of Gaussian random variable squared. Hence, $\tr[\Sigma_i]$ follows Gamma distribution with parameters $1/2$ and $2\sigma^2_x$. 
For the second term $B$, we have the following result from \citep{modelsharing2020donahue}:
\begin{align*}
    \E[B] = \frac{\mu_\epsilon}{n_i - D - 1} \cdot D
\end{align*}
For the last term $C$, we can substitute the expression from OLS and get:
\begin{align*}
    \E[C] &= 2\E_{\substack{\mu_i \sim \calN(\theta, \Sigma_\mu)\\ x \sim \calX_i}}[(x^\top \theta - x^\top \mu_i)(x^\top \mu_i - x^\top w_i)]\\
    &= 2 \E_{\substack{\mu_i \sim \calN(\theta, \Sigma_\mu)\\ x \sim \calX_i}}[(x^\top \theta - x^\top \mu_i)(- x^\top (X_i^\top X_i)^{-1} X_i^\top \eta_i)]\\
    &= -2 \E_{\substack{\mu_i \sim \calN(\theta, \Sigma_\mu)\\ x \sim \calX_i}}[x^\top (\theta - \mu_i) x^\top (X_i^\top X_i)^{-1} X_i^\top \eta_i | \mu_i]\\
    &=  -2 \E_{\substack{\mu_i \sim \calN(\theta, \Sigma_\mu)\\ x \sim \calX_i}}[x^\top (\theta - \mu_i)] \E_{x \sim \calX_i}[x^\top (X_i^\top X_i)^{-1} X_i^\top \eta_i | \mu_i]\\
    &= -2 \E_{x \sim \calX_i}[x^\top (\theta - \theta)] \E_{x \sim \calX_i}[x^\top (X_i^\top X_i)^{-1} X_i^\top \eta_i]\\
    &= 0
\end{align*}
Hence, the expectation over sum of all three terms is:
\begin{align*}
    MSE(w_i) &= \E[A] + \E[B] + \E[C]\\
    &= \tr[\Sigma_\mu \Sigma_i] + \frac{\mu_\epsilon}{n_i - D - 1} \cdot D + 0\\
    &= \tr[\Sigma_\mu \Sigma_i] + \frac{\mu_\epsilon}{n_i - D - 1} \cdot D
\end{align*}
\end{proof}

We assume that if a client $i$ join the coalition $S$, they can have access to the local models of all other participating clients in $S$. Then, client $i$ can assign a weight vector $v_{ij}$ that weights every other client $j$'s  contribution to their estimate. Formally, we have:
\begin{equation*}
    w_i^S = \sum_{j \in S} v_{ij} w_{j} 
\end{equation*}
for $\sum_{j \in S}v_{ij} = 1$. 
Then, we can calculate the expected MSE from using an aggregated model $w_i^S$:
\begin{lemma}[Fine-grained federation]
For linear regression, the expected MSE of the shared model in coalition $S$ for a client $i$ with $n_i$ samples is:
\begin{equation*}
    \mu_\epsilon \sum_{j=1}^{\abs{S}} v_{ij}^2 \frac{D}{n_j - D - 1} + \tr[\Sigma_\mu \Sigma_i] + \dncomment{Cross}
\end{equation*}
where $N = \sum_{j=1}^{\abs{S}} n_j$ is the total number of samples in the coalition. 
\end{lemma}
\begin{proof}
First, we can expand the MSE expression using definition of fine-grained federation:
\begin{align*}
    (x^\top \theta - x^\top w_S)^2 &= [(x^\top \theta - x^\top \mu_i) + ( x^\top \mu_i - x^\top w_i^S )]^2\\
    &= \underbrace{(x^\top \theta - x^\top \mu_i)^2}_{A} + \underbrace{(x^\top \mu_i - x^\top w_i^S)^2}_{B} + \underbrace{2(x^\top \theta - x^\top \mu_i)(x^\top \mu_i - x^\top w_i^S)}_C
\end{align*}
We proceed to calculate the expectation of each summand separately. For $A$, similar to the previous calculation for local estimator, we have:
\begin{align*}
    \E[A] &= \E_{\substack{\mu_i \sim \calN(\theta, \Sigma_\mu)\\ x \sim \calX_i}}[(x^\top \theta - x^\top \mu_i)^2]\\
    &= \tr[\Sigma_\mu \Sigma_i]
\end{align*}
For the second term $B$, we have the following result from \citet{modelsharing2020donahue}:
\begin{equation*}
    \E[B] = \mu_\epsilon \sum_{j=1}^{\abs{S}} v_{ij}^2 \frac{D}{n_j - D - 1}
\end{equation*}
where $N = \sum_{j=1}^{\abs{S}} n_j$ and $\mu_\epsilon = \E_{\epsilon}[\epsilon_i^2]$. 
For the last term $C$, we can substitute the expression of $w_S$ from fine-grained federation and get:
\begin{align*}
    \E[C] &= 2 \E_{\substack{\mu_i \sim \calN(\theta, \Sigma_\mu)\\ x \sim \calX_i \\ X_j \sim \calX_j}}[(x^\top \theta - x^\top \mu_i)(x^\top \mu_i - x^\top w_i^S)]\\
    &= 2 \E_{\substack{\mu_i \sim \calN(\theta, \Sigma_\mu)\\ x \sim \calX_i\\ X_j \sim \calX_j}} \left[x^\top (\theta - \mu_i)x^\top \left(\mu_i - \sum_{j \in S} v_{ij} w_j \right) \right]\\
    &= 2\E_{\substack{\mu_i \sim \calN(\theta, \Sigma_\mu)\\ x \sim \calX_i \\ X_j \sim \calX_j}} \left[x^\top (\theta - \mu_i) x^\top \left( \mu_i - \E \left[\sum_{j \in S} v_{ij} w_j \Bigg| \mu_i \right]  \right) \right]\\
    &= 2 \E_{\substack{\mu_i \sim \calN(\theta, \Sigma_\mu)\\ x \sim \calX_i\\ X_j \sim \calX_j}} \left[ x^\top (\theta - \mu_i) x^\top \left( \mu_i - \sum_{j \in S} v_{ij} \mu_j \right) \right]\\
    &= 2 \E_{\substack{\mu_i \sim \calN(\theta, \Sigma_\mu) \\ x \sim \calX_i \\ X_j \sim \calX_j }} \left[ x^\top (\theta - \mu_i) x^\top \left( (1 - v_{ii}) \mu_i - \sum_{j\in S, j \neq i} v_{ij} \mu_j \right) \right]\\
    &= 2 \E_{\substack{\mu_i \sim \calN(\theta, \Sigma_\mu) \\ x \sim \calX_i \\ X_j \sim \calX_j }} \left[ x^\top (\theta - \mu_i) x^\top \left( \left(\sum_{j \in S} v_{ij} - v_{ii} \right) \mu_i - \sum_{j \in S, j \neq i} v_{ij} \mu_j \right) \right]\\
    &= 2 \E_{\substack{\mu_i \sim \calN(\theta, \Sigma_\mu) \\ x \sim \calX_i \\ X_j \sim \calX_j }} \left[ x^\top (\theta - \mu_i) x^\top \sum_{j \in S, j \neq i} v_{ij}  (\mu_i - \mu_j) \right]
\end{align*}
Taking expectation over all $\mu_j$, we have:
\begin{align*}
    \E[C] &=2 \E_{\substack{\mu_i \sim \calN(\theta, \Sigma_\mu) \\ x \sim \calX_i \\ X_j \sim \calX_j }} \left[ x^\top (\theta - \mu_i) x^\top \sum_{j \in S, j \neq i} v_{ij}  (\mu_i - \mu_j) \right] \\ 
    &= 2 \sum_{j \in S, j \neq i} v_{ij} \E_{\substack{\mu_i, \mu_j \sim \calN(\theta, \Sigma_\mu) \\ x \sim \calX_i \\ j \in S, j \neq i}}\left[ x^\top (\theta - \mu_i) x^\top (\mu_i - \mu_j) \right]\\
    &= 2 \sum_{j \in S, j \neq i} v_{ij} \E_{\substack{\mu_i, \mu_j \in \calN(\theta, \Sigma_\mu) \\ x \sim \calX_i \\ j \in S, j \neq i}}[x^\top \theta x^\top (\mu_i - \mu_j)] - 2 v_{ij} \E_{\substack{\mu_i, \mu_j \in \calN(\theta, \Sigma_\mu) \\ x \sim \calX_i \\ j \in S, j \neq i}}[ x^\top \mu_i x^\top ( \mu_i - \mu_j) ]\\
    &= 2 \sum_{j \in S, j \neq i} v_{ij} \E_{\substack{\mu_i, \mu_j \in \calN(\theta, \Sigma_\mu) \\ x \sim \calX_i \\ j \in S, j \neq i}}[ x^\top \mu_i x^\top ( \mu_j - \mu_i) ]\\
    &= 2 \sum_{j \in S, j \neq i} v_{ij} \E_{\substack{\mu_i, \mu_j \in \calN(\theta, \Sigma_\mu) \\ x \sim \calX_i \\ j \in S, j \neq i}}[x^\top \mu_i x^\top \mu_j - x^\top \mu_i x^\top \mu_i]\\
    &= 2 \sum_{j \in S, j \neq i} v_{ij} \E_{x \sim \calX_i}[x^\top \theta x^\top \theta] - v_{ij} \E_{x \sim \calX_i}[x^\top \theta x^\top \theta]\\
    &= 0
\end{align*}
\end{proof}

Then, we can derive the expected utility gain for a client $i$ joining coalition $S$ with fine-grained federation as the difference in expected error between using only local samples $w_i$ and using an aggregated model $w_i^S$:
\begin{lemma}[Utility gain linear regression]
For linear regression, the expected utility gain of joining a coalition $S$ for a client $i$ with $n_i$ samples is:
\begin{align*}
     u_i = \frac{\mu_\epsilon}{n_i - D - 1} D - \mu_\epsilon \sum_{j=1}^{\abs{S}} v_{ij}^2 \frac{D}{n_j - D - 1} - \dncomment{cross}
\end{align*}
\end{lemma}
If all clients have the same number of local samples $n = n_i \forall i$, then the expected utility gain for linear regression can be reduced to:
\begin{lemma}[Utility gain linear regression under fixed $n_i$]
For linear regression where all clients have the same number of local samples $n$, the expected utility gain of joining a coalition $S$ for a client $i$ is:
\begin{equation*}
    u_i =  \frac{\mu_\epsilon \cdot D}{n - D - 1} \cdot \left(1 - \sum_{j=1}^{\abs{S}} v_{ij}^2  \right)
\end{equation*}
\end{lemma}
Hence, for a client $i$ to determine whether it is beneficial or not to join a coalition $S$, they first need to determine the optimal weights $v_{ij}$ for each participating client $j$. In the most extreme case, where the client $i$ does not trust other clients' local model, they can place all the weight on their own estimate, \ie $v_{ii} = 1$ and $0$ weight for all other models, \ie $v_{ij} = 0, \forall j \in S, j \neq i$. Then, the utility gain from joining the coalition $S$ is exactly $0$, and client $i$ would not join since they would incur some positive loss $c_i > 0$.  

%%%%%% Alternative definition %%%%%%%
All clients want to learn a shared global parameter $\theta$. Since there is only one grand coalition $S$ in the population, we assume that all clients who join the coalition will share an estimator formed by the fine-grained federation. That is, for all clients $j \in S$, the weight vector $v_j$ is fixed and shared across the coalition. This weight vector is calculated by performing an optimization task over the expected utility gain.
