# Supplementary material for: Federated Learning as a Network Effects Game
Source: arXiv:2302.08533 source file (2023-02-16)
Supplement: Supplementary file 2 [file personalized.tex]

\section{Personalized Setting}
Every client $i$ has a mean vector $\mu_i \in \mathbb{R}^d$, which is $k$-sparse, i.e. $\mu_i$ has support of size $k$. Each client $i$ has $n_i$ data points $x_{ij} \in \mathbb{R}^d$ for $j = 1, \cdots, n_i$. Each data point is determined by $x_{ij} = \mu_i + z_{ij}$, where $z_{ij}$ is a noise vector drawn independently from a $\eta_i$-sub-Gaussian distribution. We assume all mean vectors $\mu_i$ share the same support $S$. Then, without joining the coalition, the estimated mean $\mu^{(i)}$ using only local data is the empirical average of all local data samples $x_{ij}$:  
\begin{equation*}
    \hat{\mu}_i = \frac{1}{n_i} \sum_{j=1}^{n_{i}} x_{ij}
\end{equation*}
Similar to the non-personalized setting, we calculate the expected error of $\hat{\mu}_i$ at a particular test point $x$: when the expectation is taken over all $x \sim \calX_i$, it represents the average error everywhere on the distribution. Hence, the expected estimation error for using only local data is:
\begin{align*}
    \E[(x^\top \mu_i - x^\top \hat{\mu}_i)^2] &= \frac{\eta_i}{n_i}
\end{align*}
\begin{proof}
First, we look at the expression inside the expectation. Substituting in the definition of local estimator $\hat{\mu}_i$, we have:
\begin{align*}
    (x^\top \mu_i - x^\top \hat{\mu}_i)^2 &= \left[ x^\top \mu_i - x^\top \left( \frac{1}{n_i} \sum_{j=1}^{n_i} x_{ij} \right) \right]^2\\
    &= \left[ x^\top \left( \mu_i - \frac{1}{n_i} \sum_{j=1}^{n_i} x_{ij} \right) \right]^2\\ 
    &= \left[ x^\top \left(\mu_i - \frac{1}{n_i} \left( \sum_{j=1}^{n_i} \mu_i + z_{ij} \right) \right) \right]^2\\
    &= \left[ x^\top \left( - \frac{1}{n_i} \sum_{j=1}^{n_i} z_{ij} \right) \right]^2\\
    &= \left(\frac{1}{n_i} \sum_{j=1}^{n_i} x_{ij} \right)^\top x x^\top \left(\frac{1}{n_i} \sum_{j=1}^{n_i} x_{ij} \right)\\
    &= \tr\left[ \left(\frac{1}{n_i} \sum_{j=1}^{n_i} x_{ij} \right)^\top x x^\top \left(\frac{1}{n_i} \sum_{j=1}^{n_i} x_{ij} \right) \right]\\
    &= \tr\left[x x^\top \left(\frac{1}{n_i} \sum_{j=1}^{n_i} x_{ij} \right)  \left(\frac{1}{n_i} \sum_{j=1}^{n_i} x_{ij} \right)^\top \right]
\end{align*}
Note that in the last three steps, we use the fact that for a scalar $c$, we have $c = \tr[c]$ and the cyclic property of trace to reorder the matrix product. Then, we can apply expectation over all test point $x$ and get:
\begin{align}
    \E_{x \sim \calN(\mu_i, \eta_i)}[x^\top \mu_i - x^\top \hat{\mu}_i] &= \tr\left[ \E_{x \sim \calN(\mu_i, \eta_i)}[xx^\top] \left(\frac{1}{n_i} \sum_{j=1}^{n_i} x_{ij} \right) \left( \frac{1}{n_i} \sum_{j=1}^{n_i} x_{ij} \right)^\top \right]\\
    &= \tr \left[ \Sigma_i \left( \frac{1}{n_i} \sum_{j=1}^{n_i} x_{ij} \right) \left( \frac{1}{n_i} \sum_{j=1}^{n_i} x_{ij} \right)^\top \right]
\end{align}
where $\Sigma_i = \E_{x \sim \calX_i}[xx^\top]$. Applying expectation over the samples $x_{ij}$, we get:
\begin{align*}
    \E_{x_{ij} \sim \calN(\mu_i, \eta_i)} [x^\top \mu_i - x^\top \hat{\mu}_i] &= \tr \left[ \Sigma_i \E_{x_{ij} \sim \calN(\mu_i, \eta_i)} \left[\left( \frac{1}{n_i} \sum_{j=1}^{n_i} x_{ij} \right) \left( \frac{1}{n_i} \sum_{j=1}^{n_i} x_{ij} \right)^\top\right] \right]\\
    &= \tr[\Sigma_i \E_{x_{ij} \sim \calN(\mu_i, \eta_i)}[M]] 
\end{align*}
where $M = \left( \frac{1}{n_i} \sum_{j=1}^{n_i} x_{ij} \right) \left( \frac{1}{n_i} \sum_{j=1}^{n_i} x_{ij} \right)^\top$. Note that $M$ is a $d\times d$ matrix, where the $\ell$-th diagonal entry is $\left(\nicefrac{1}{n_i} \sum_{j=1}^{n_i} x_{ij}^{(\ell)} \right)^2$ which has expectation $\eta_i$. The off-diagonal entries are $\left( \nicefrac{1}{n_i} \sum_{j=1}^{n_i} x_{ij}^{\ell} \right) \cdot \left( \nicefrac{1}{n_i} \sum_{j=1}^{n_i} x_{ij}^{k} \right)$ for $\ell \neq k$. Since the noise for each data point is drawn independently from a zero-mean distribution, the expectation of each off-diagonal entry is $0$. 
\end{proof}
%%%%% New stuff %%%%%%%
\dncomment{PCA starts here}

When the client instead use pooled data from the coalition, they can identify the support of $\mu_i$ to get a better estimate by using PCA. Let $N_S$ denote the total number of samples in the coalition. Let $X_i \in \mathbb{R}^{d \times n}$ denote the matrix containing data samples from client $i$. Then, we can write $X_i = M + Z$, where the $i$-th column of $M$ is the mean vector $\mu_i$, and $Z$ is the noise matrix where each coordinate is drawn independently from a $\eta_i$-sub-Gaussian distribution. First, we decompose $X$ into $U \Sigma V^\top$, where $U$ is a $d \times d$ unitary matrix, $\Sigma$ is a $d \times n$ rectangular diagonal matrix and $V$ is a $n \times n$ unitary matrix. The columns of $U$ are the left singular vectors of $X$, the diagonal entries of $\Sigma$ are the singular values of $X$, and the columns of $V$ are the right singular vectors of $X$. Using this decomposition, we can show that $X^\top X = V \Lambda V^\top$, where $\Lambda \in \mathbb{R}^{d \times d}$ is a diagonal matrix with non-zero eigenvalues of $X^\top X$.
